# Supplementary material for: A Geometric Analysis of Neural Collapse with Unconstrained Features
Source: arXiv:2105.02375 source file (2021-05-06)
Supplement: Supplementary file 1 [file main_theory-save-March28.tex]

\subsection{Proof of \Cref{thm:global-minima}}

We first characterize the following balance property between $\mW$ and $\mH$ for any critical point  $(\mW,\mH)$ of \eqref{eq:obj}.
\begin{lemma} Any critical point $(\mW,\mH)$ of \eqref{eq:obj} obeys
\e
\mW^\top\mW = \frac{\lambda_{\mH}}{\lambda_{\mW}}\mH\mH^\top.
\label{eq:critical-balance}\ee	
\label{lem:critical-balance}\end{lemma}
\begin{proof}[Proof of \Cref{lem:critical-balance}]
	Any critical point $(\mW,\mH)$ of \eqref{eq:obj} satisfies
	\begin{align*}
	&\nabla_{\mW}f(\mW,\mH) = \nabla g(\mW\mH)\mH^\top + \lambdaW \mW = \vzero,\\
	&\nabla_{\mH}f(\mW,\mH) =  \mW^\top g(\mW\mH) + \lambdaW \mH = \vzero.	
	\end{align*}
Multiplying the first equation from the left with $\mW^\top$ and the second equation from the right with $\mH^\top$, and combining them together give
\[
\lambdaW \mW^\top \mW = \lambdaH \mH \mH^\top.
\]
\end{proof}

We now turn to prove \Cref{thm:global-minima}. 
Similar to \cite{lu2020neural,fang2021layer}, we prove \Cref{thm:global-minima} by directly showing that $f(\mW,\mH)> f(\mW^*,\mH^\star)$ for all $\mW,\mH$ that are not the form of \eqref{eq:global-minima}.
\begin{proof}[Proof of \Cref{thm:global-minima}] First note that the objective function $f$ is coercive since the cross-entropy is always nonnegative, implying that the global minimizer of \eqref{eq:obj} is always finite. By \Cref{lem:critical-balance}, we only need to consider all the points that $\mW^\top\mW = \frac{\lambda_{\mH}}{\lambda_{\mW}}\mH\mH^\top$. To simplify the notation, let  $\|\mW\|_F^2 = \rho$, and thus $\|\mH\|_F^2 = \frac{\lambda_{\mH}}{\lambda_{\mW}}\rho$. We will first provide a lower bound for the cross-entropy term for any $\mW$  with energy $\rho$. Towards that goal, note that for any $\vz\in\R^{K}$, the cross-entropy loss with $\vy_k$ can be lower bounded by
\e\begin{split}
	&\calL(\vz,\vy_k) =  \log\bracket{\frac{\sum_{j=1}^K \exp\bracket{z_j}}{\exp\bracket{z_k}}} = \log\bracket{1 + \sum_{j\neq k} \exp\bracket{z_j - z_k}}\\
	& \ge \log\bracket{1 + (K-1) \exp\bracket{\sum_{j\neq k}\frac{z_j - z_k}{K-1}}} \\
	&= \log\bracket{1 + (K-1) \exp\bracket{\frac{\bracket{\sum_{j=1}^K z_j} -K  z_k}{K-1}}}\\
	& \ge  \frac{1}{1+c_1}\log\bracket{(1+c_1)(K-1) \exp\bracket{\frac{\bracket{\sum_{j=1}^K z_j} -K  z_k}{K-1}}  } + \frac{c_1}{1+c_1}\log\bracket{\frac{1+c_1}{c_1}}\\
	& = \frac{1}{1+c_1} \frac{\bracket{\sum_{j=1}^K z_j} -K  z_k}{K-1} + \underbrace{\frac{1}{1+c_1}\log\bracket{(1+c_1)(K-1)} +  \frac{c_1}{1+c_1}\log\bracket{\frac{1+c_1}{c_1}}  }_{c_2},
\end{split}\label{eq:cross-entropy-lower-bound}\ee
where the first inequality follows from the Jesen's inequality for $\sum_{j\neq k} \exp\bracket{z_j - z_k}$ and it achieves the equality only when $\vz_j = \vz_i$ for all $i,j\neq k$, and we set $c_1 = \frac{1}{(K-1)\exp\bracket{-\frac{\rho}{K-1}\sqrt{\frac{\lambdaH}{\lambdaW n}}}}$ in the second inequality which follows because the concavity of the $\log$ function (i.e., $\log\bracket{t x + (1-t)y} \ge t\log x + (1-t)\log y$ for any $t\in[0,1]$) and achieves its equality when $(K-1) \exp\bracket{\sum_{j\neq k}\frac{z_j - z_k}{K-1}} = \frac{1}{c_1}$.

We now using \eqref{eq:cross-entropy-lower-bound} to obtain a lower bound for $g(\mW,\mH)$ as
\e\begin{split}
    &g(\mW,\mH) - Nc2 \ge \frac{1}{(1+c_1)(K-1)} \sum_{i=1}^n\sum_{k=1}^K\bracket{ \sum_{j=1}^K\vw_j^\top \vh_{k,i} - K \vw_k^\top \vh_{k,i}  }\\
    & = \frac{1}{(1+c_1)(K-1)} \sum_{i=1}^n \bracket{ \sum_{k=1}^K\vw_k^\top \bracket{\sum_{j=1}^K\vh_{j,i}} - K \sum_{k=1}^K\vw_k^\top \vh_{k,i}  }\\
    & = \frac{K}{(1+c_1)(K-1)} \sum_{i=1}^n  \sum_{k=1}^K\vw_k^\top \bracket{\overline \vh_i -\vh_{k,i}}\\
    & \ge - \frac{nKc_3}{2(1+c_1)(K-1)}  \sum_{k=1}^K\norm{\vw_k}{2}^2 - \frac{K}{2c_3(1+c_1)(K-1)} \sum_{i=1}^n  \sum_{k=1}^K \norm{\overline \vh_i -\vh_{k,i}}{2}^2 \\
    & = - \frac{nKc_3}{2(1+c_1)(K-1)}  \sum_{k=1}^K\norm{\vw_k}{2}^2 - \frac{K}{2c_3(1+c_1)(K-1)} \sum_{i=1}^n  \bracket{\sum_{k=1}^K \norm{\vh_{k,i}}{2}^2 - K\norm{\overline \vh_i}{2}^2}\\
    & \ge - \frac{nKc_3}{2(1+c_1)(K-1)}   \rho - \frac{K}{2c_3(1+c_1)(K-1)} \frac{\lambda_{\mH}}{\lambda_{\mW}}\rho
\end{split}
\label{eq:all-cross-entropy-lower-bound}\ee
where $\overline \vh_i  = \frac{1}{K} \sum_{k=1}^K \vh_{k,i}$, $c_3 = \sqrt{\frac{\lambda_{\mH}}{n\lambda_{\mW}}}$, the second inequality follows from the Cauchy–Schwarz inequality and achieves its equality when $c_3\vw_k = (\vh_{k,i} - \overline\vh_i)$ for all $k\in[K],i\in[n]$, and the last inequality achieves its equality when $\overline \vh_i = \vzero$ for all $i\in[n]$.

Applying \eqref{eq:all-cross-entropy-lower-bound} to the objective function \eqref{eq:obj}, we have
\e\begin{split}
    f(\mW,\mH) &\ge - \frac{c_3}{2(1+c_1)(K-1)}   \rho - \frac{1}{2nc_3(1+c_1)(K-1)} \frac{\lambda_{\mH}}{\lambda_{\mW}}\rho + c_2 + \frac{\lambdaW}{2}\rho + \frac{\lambdaH^2}{2\lambdaW}\rho\\
    &= \underbrace{- \frac{1}{(1+c_1)(K-1)}\sqrt{\frac{\lambda_{\mH}}{n\lambda_{\mW}}}   \rho  + c_2 + \frac{\lambdaW}{2}\rho + \frac{\lambdaH^2}{2\lambdaW}\rho}_{\xi(\rho;\lambdaW,\lambdaH)}. 
\end{split}
\label{eq:obj-lower-boound}\ee
Note that for any fixed $\lambdaW,\lambdaH>0,$ we have $(i)$ $c_1 = \frac{1}{(K-1)\exp\bracket{-\frac{\rho}{K}\sqrt{\frac{\lambdaH}{\lambdaW}}}}$ is an increasing function in terms of $\rho$, $c_2 = \frac{1}{1+c_1}\log\bracket{(1+c_1)(K-1)} +  \frac{c_1}{1+c_1}\log\bracket{\frac{1+c_1}{c_1}}$ is a decreasing function in terms of $c_1$, 
$(ii)$ $c_1  \rightarrow \frac{1}{K-1}$ and $c_2 \rightarrow \log K$ when $\rho\rightarrow 0$, and $(iii)$ $c_1  \rightarrow \infty$ and $c_2 \rightarrow 0$ when $\rho\rightarrow 0$. Thus, as plotted in \Cref{fig:obj-lower-bound}, 
$\xi(\rho;\lambdaW,\lambdaH) \rightarrow \log K$ when $\rho\rightarrow 0$ and $\xi(\rho;\lambdaW,\lambdaH) \rightarrow \infty$ when $\rho\rightarrow \infty$, and $\xi(\rho;\lambdaW,\lambdaH)$ achieves its minimum at a finite $\rho$.

\begin{figure}[htp!]
	\centering
    \includegraphics[width = 0.6\textwidth]{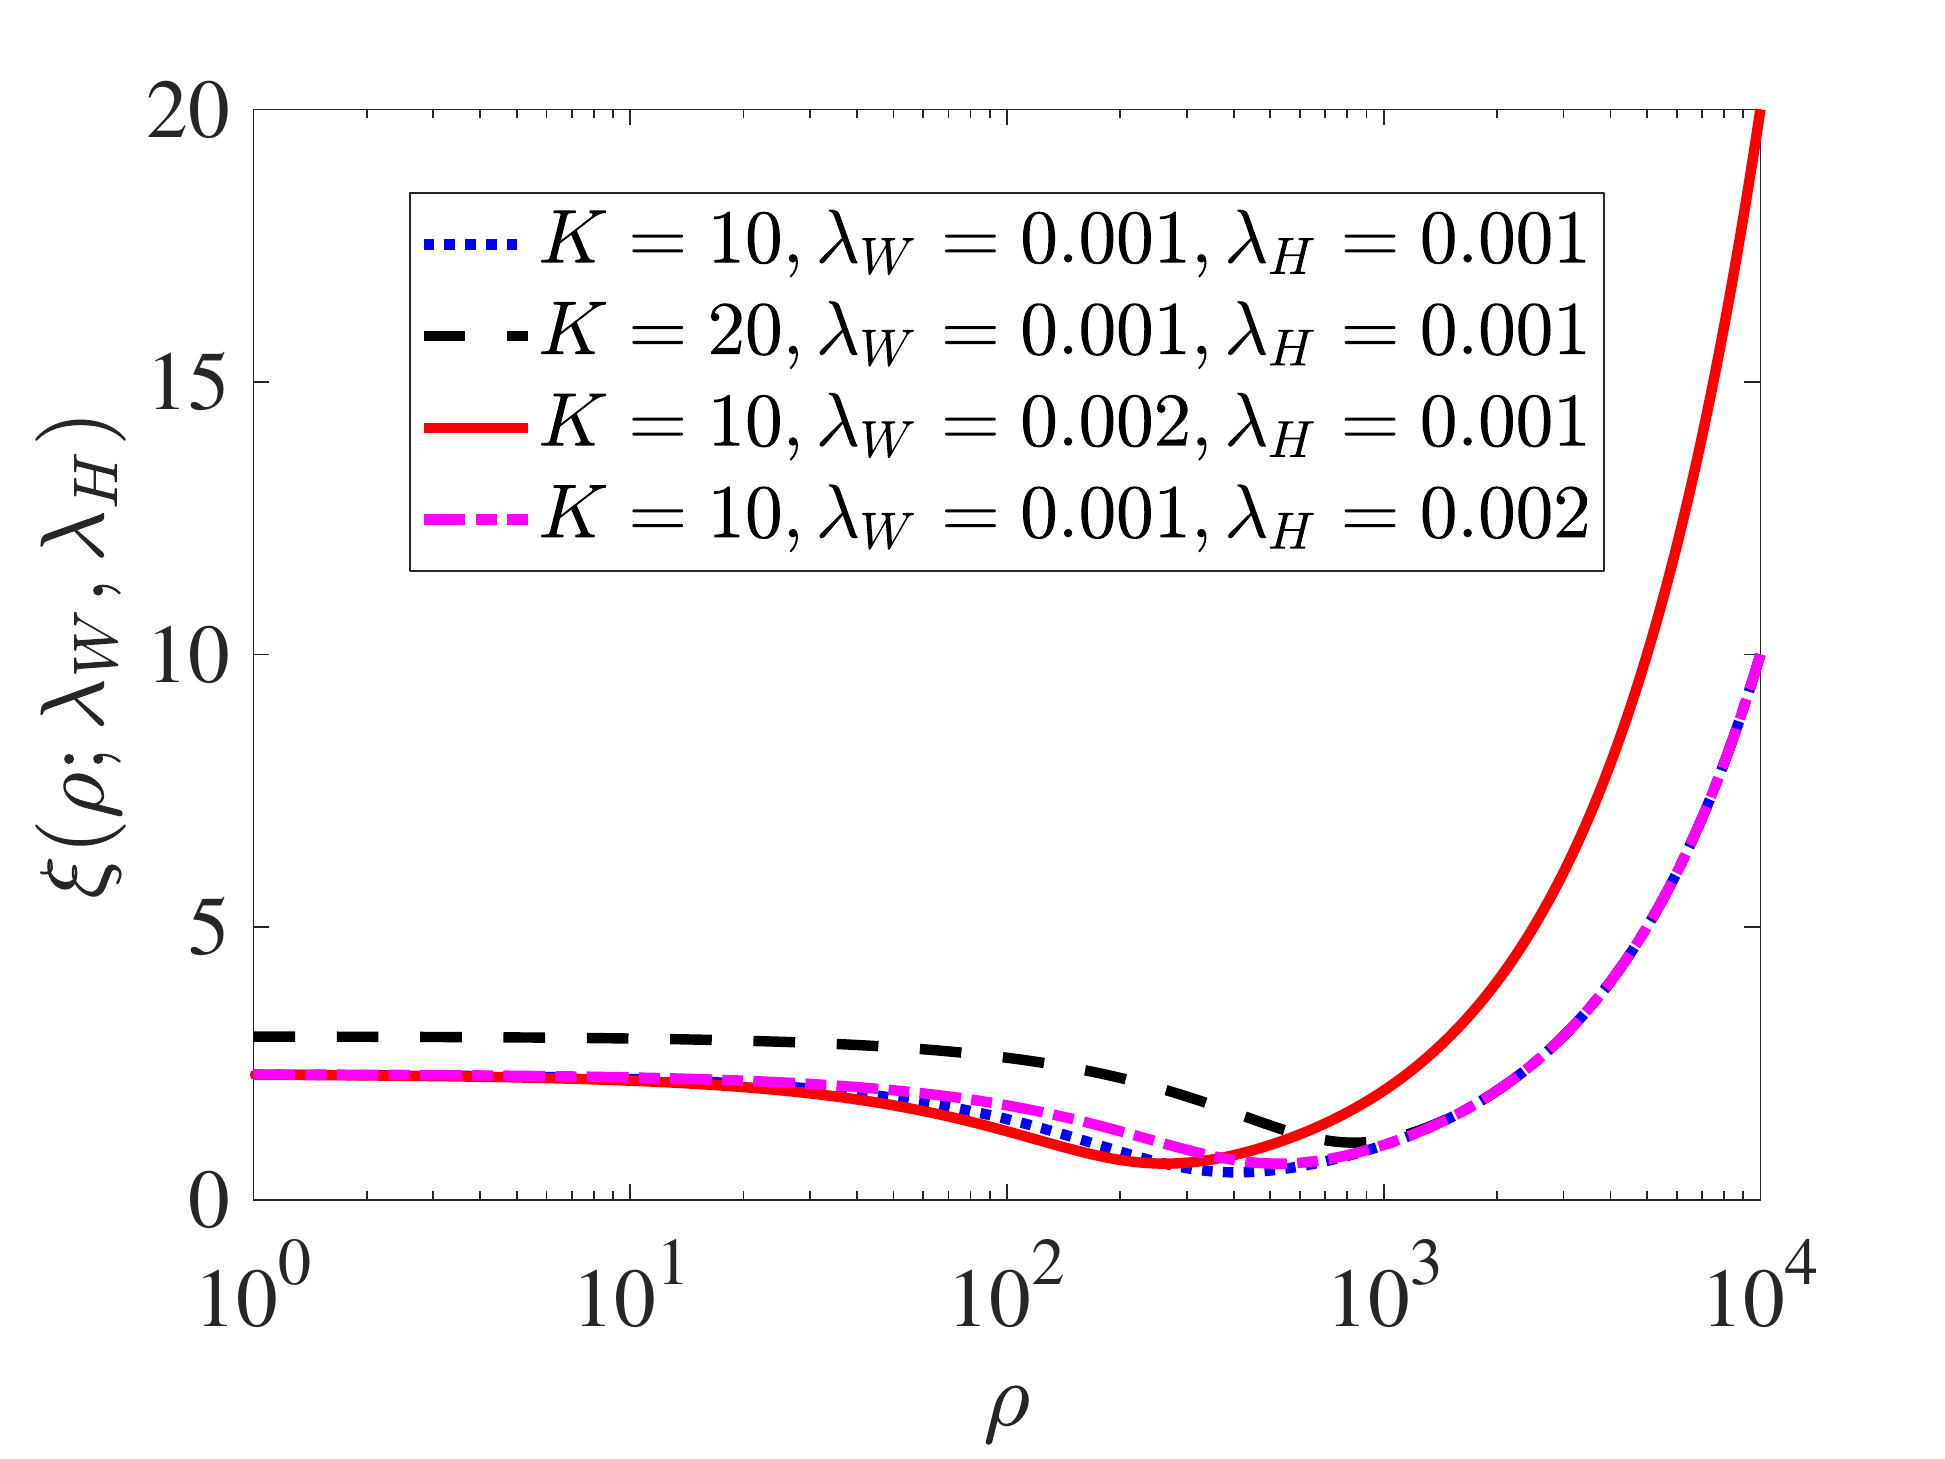}
	\caption{Plot of $\xi(\rho;\lambdaW,\lambdaH)$ in terms of $\rho$ for $\lambdaW = \lambdaH = 10^{-3}$, $K = 10$, and $n = 100$.}
	\label{fig:obj-lower-bound}
\end{figure}

One can verify that all the inequalities in \eqref{eq:cross-entropy-lower-bound} and \eqref{eq:all-cross-entropy-lower-bound} (and hence \eqref{eq:obj-lower-boound}) achieve equality when $\mW$ and $\mH$ have the form as in \Cref{thm:global-minima}. The remaining of the proof is to show the equalities are only achieved when $\mW$ and $\mH$ have the form as in \Cref{thm:global-minima}. Towards that goal, assume $(\mW,\mH)$ is a global minimizer of \eqref{eq:obj}, hence \eqref{eq:cross-entropy-lower-bound}, \eqref{eq:all-cross-entropy-lower-bound}, and \eqref{eq:obj-lower-boound} obtain the equality at this point. We first recall that  \eqref{eq:all-cross-entropy-lower-bound} achieving equality requires $c_3\vw_k = (\vh_{k,i} - \overline\vh_i)$ and $\overline \vh_i = \vzero$ for all $k\in[K],i\in[n]$, which further implies that $\vh_{k,i} = c_3 \vw_k$ for all $k\in[K],i\in[n]$. Moreover, to achieve its equality for the first line of \eqref{eq:all-cross-entropy-lower-bound}, it requires 
\[
c_3(\sum_{j=1}^K\vw_j^\top)\vw_k - c_3K \vw_k^\top \vw_k = (K-1)\log\frac{1}{c_1(K-1)}, \quad \forall k\in[K].
\]
This together with the fact $\overline\vh_i = c_3 (\sum_{j=1}^K \vw_j) = \vzero$ gives  
\[
\|\vw_k\|_2^2 = -\frac{(K-1)}{c_3 K}\log\frac{1}{c_1(K-1)} =  \frac{\rho}{K}
\]
for all $k\in[K]$. To achieve its equality for the first line of \eqref{eq:all-cross-entropy-lower-bound}, it also requires $\vw_{j}^\top \vw_{k} = \vw_{j'}^\top \vw_{k}$ for all $j,j'\neq k$, $k\in[K]$. Combining this together with the fact $\sum_{j=1}^K \vw_j^\top \vw_k = 0$ gives 
\[
\vw_j^\top \vw_k = -\frac{\rho}{K(K-1)}
\]
for all $j,k\in[K]$ and $j\neq k$. Thus, we complete the proof by noting that
\[
\mW\mW^\top = \frac{\rho}{K-1}\bracket{\mId_K - \vone_K\vone_K^\top}
\]
which implies the scaled version of $\mW^\top$ forms a simplex ETF.
\end{proof}

\subsection{Proof of \Cref{thm:global-geometry}}

Denote by $\alpha = \frac{\lambda_{\mH}}{\lambda_{\mW}}$. The following Lemma extends the standard variational form of nuclear norm.

\begin{lemma} For any $\mX\in\R^{K\times N}$, we have
\[
\|\mX\|_* = \min_{\mX =\mU\mV} \frac{1}{2\sqrt{\alpha}}\bracket{\|\mU\|_F^2 + \alpha\|\mV\|_F^2}.
\]
	
\end{lemma}

Thus, we can view \eqref{eq:obj} as the bilinear factorization problem of
\e
\min_{\mZ\in\R^{K\times N}}\xi(\mZ) = g(\mZ) + \sqrt{\alpha}\lambda_{\mW}\|\mZ\|_*.
\label{eq:convex-prob}\ee

As in \cite{li2019non}, we will characeterize the critical points of \eqref{eq:obj} by establishing the connection to the optimality condition of the convex problem \eqref{eq:convex-prob}.
  
\begin{lem}[Optimality condition] If critical point $(\mW,\mH)$ of \eqref{eq:obj} satisfies
\[
\|\nabla g(\mW\mH)\| \le \sqrt{\lambdaW\lambdaH},
\]
then it is a global minimum of \eqref{eq:obj}.	
\end{lem}

\begin{lem}[Optimality condition] If critical point $(\mW,\mH)$ of \eqref{eq:obj} satisfies
\[
\|\nabla g(\mW\mH)\| > \sqrt{\lambdaW\lambdaH},
\]
then it is a strict saddle.	
\label{lem:strict saddle}\end{lem}
\begin{proof}[Proof of \Cref{lem:strict saddle}] For any $\mDelta = (\mDelta_{\mW},\mDelta_{\mH})$, the Hessian bilinear form of $f$ along the direction $\mD$ is given by
\begin{align*}
\nabla f(\mW,\mH)[\mDelta,\mDelta] =& 2\innerprod{\nabla g(\mW\mH)}{\mDelta_{\mW}\mDelta_{\mH}} + [\nabla^2g(\mW\mH)](\mW\mDelta_{\mH} + \mDelta_{\mW}\mH,\mW\mDelta_{\mH} + \mDelta_{\mW}\mH) \\
&+ \lambdaW\|\mDelta_{\mW}\|_F^2 + \lambdaH\|\mDelta_{\mH}\|_F^2.
\end{align*}

We now utilize the assumption that $\|\nabla g(\mW\mH)\| > \sqrt{\alpha}\lambda_{\mW}$ to construct a negative curvature direction. Towards that goal, let $\vp$ and $\vq$ are the left and right singular vectors corresponding to its largest singular value, which is larger than $\sqrt{\alpha}\lambda_{\mW}$ by assumption.

Since $d>K$, there exists a nonzero $\va\in\R^{d}$ in the null space of $\mW$, i.e., $\mW\va = 0$. It follows from \Cref{lem:critical-balance} that $\mW^\top\mW = \alpha\mH\mH^\top$, which further implies that $\mH^\top\va = \vzero$. We now construct the negative curvature direction as $\mDelta_{\mW} = \alpha^{1/4} \vp \va^\top$ and $\mDelta_{\mH} = -\frac{1}{\alpha^{1/4}} \va \vq^\top$. Noting that 
\[
\mW\mDelta_{\mH} + \mDelta_{\mW}\mH = -\frac{1}{\alpha^{1/4}}\mW  \va \vq^\top +  \alpha^{1/4} \vp \va^\top \mH = \vzero,
\]
we have
\begin{align*}
\nabla f(\mW,\mH)[\mDelta,\mDelta] &= 2\innerprod{\nabla g(\mW\mH)}{\mDelta_{\mW}\mDelta_{\mH}} + \lambdaW\|\mDelta_{\mW}\|_F^2 + \lambdaH\|\mDelta_{\mH}\|_F^2\\
& = -2\|\va\|^2\innerprod{\nabla g(\mW\mH)}{\vp\vq^\top} + \lambdaW\sqrt{\alpha} \|\va\|^2 + \frac{\lambdaH}{\sqrt{\alpha}}\|\va\|^2\\
& = -2\|\va\|^2 \bracket{\|\nabla g(\mW\mH)\| - \sqrt{\lambdaW\lambdaH}} <0
\end{align*}
since by assumption $\|\nabla g(\mW\mH)\| > \sqrt{\lambdaW\lambdaH}$.
	
\end{proof}
